# Supplementary material for: PAI-graphene: a new topological semimetallic two-dimensional carbon allotrope with highly tunable anisotropic Dirac cones
Source: arXiv:2007.12251 source file (2020-07-23)
Supplement: Supplementary file 1 [file SI.pdf]

*Support Information for*

# PAI-graphene: a new topological semimetallic two-dimensional carbon allotrope with highly tunable anisotropic Dirac cones

Xin Chen,[1] Adrien Bouhon, [2,1] Linyang Li, [3, 4]* François M. Peeters, [5,4] and Biplab Sanyal[1, *]

[1]Department of Physics and Astronomy, Uppsala University, Box 516, 751 20 Uppsala, Sweden

[2]Nordic Institute for Theoretical Physics (NORDITA), Stockholm, Sweden

[3]School of Science, Hebei University of Technology, Tianjin 300401, People's Republic of China

[4]Department of Physics, University of Antwerp, Groenenborgerlaan 171, B-2020 Antwerp, Belgium

[5]Department of Physics and Astronomy, Key Laboratory of Quantum Information of Yunnan Province, Yunnan University, 650091 Kunming, China

Corresponding authors:

*Email: linyang.li@hebut.edu.cn (L. L.)

*Email: biplab.sanyal@physics.uu.se (B. S.)

I. BOMD simulations at 300 K and 800 K

To investigate the thermal stability of PAI-graphene, we performed BOMD simulations at 300 K, 800 K, and 1500 K with a time step of 1 fs. The results for BOMD at 1500 K are shown in Figure 2(d), and the results for that at 300 K and 800 K are shown in Figure S1.

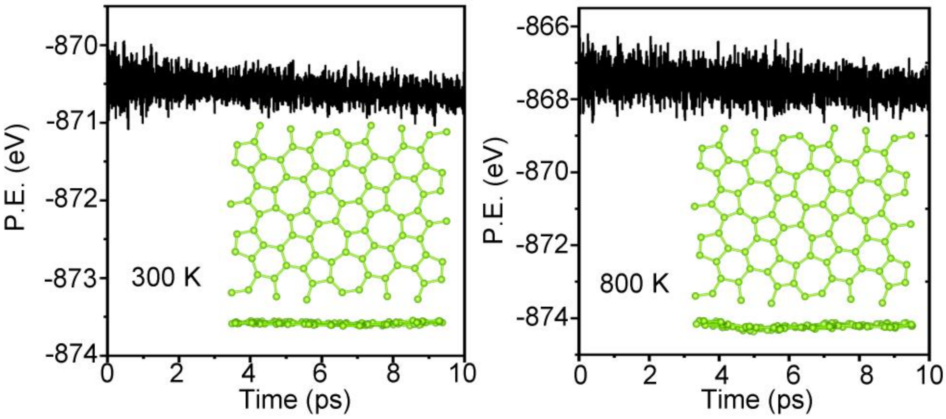


Figure S1 Potential energy (P.E.) as a function of BOMD simulation time at 300 K and 800 K, and the top and side view of the final structures.

II. Strain-induced insulating properties of PAI-graphene

The electronic band structures of PAI-graphene under strain $(\tau_x, \tau_y) = (8\%, 10\%)$ and $(\tau_x, \tau_y) = (9\%, 10\%)$ as shown by the blue dots in Figure 4(a) are shown in Figure S2.

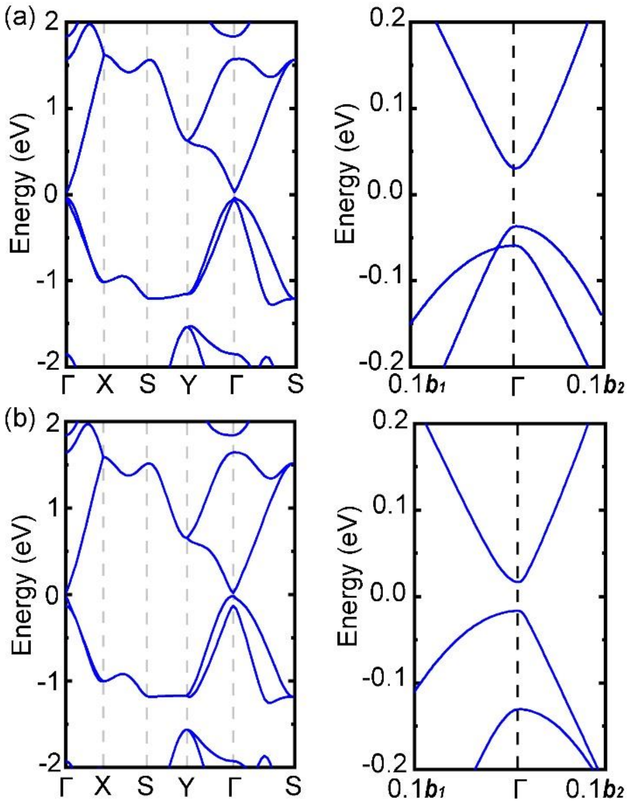


Figure S2 The band structures of PAI-graphene under strain (a) $(\tau_x, \tau_y) = (8\%, 10\%)$, and (b) $(\tau_x, \tau_y) = (9\%, 10\%)$. $\boldsymbol{b_1}$ and $\boldsymbol{b_2}$ are the reciprocal lattice vectors as shown in Figure 2(a).

## III. Position of atoms in PAI-graphene

The obtained POSCAR of PAI-graphene is:

```
PAI-graphene
1.00000000000000
8.99507430   0.00000000   0.00000000
0.00000000   7.20572025   0.00000000
0.00000000   0.00000000   21.70617435
C
24
Direct
0.68157953   0.37376692   0.50000000
0.31842047   0.62623308   0.50000000
0.81842047   0.87376692   0.50000000
0.18157953   0.12623308   0.50000000
0.93586545   0.44595710   0.50000000
0.06413455   0.55404290   0.50000000
0.56413455   0.94595710   0.50000000
0.43586545   0.05404290   0.50000000
0.97400100   0.90354111   0.50000000
0.02599900   0.09645889   0.50000000
0.52599900   0.40354111   0.50000000
0.47400100   0.59645889   0.50000000
0.73556633   0.70332252   0.50000000
0.26443367   0.29667748   0.50000000
0.76443367   0.20332252   0.50000000
0.23556633   0.79667748   0.50000000
0.91980683   0.24328037   0.50000000
0.08019317   0.75671963   0.50000000
0.58019317   0.74328037   0.50000000
0.41980683   0.25671963   0.50000000
0.78563750   0.52051967   0.50000000
0.21436250   0.47948033   0.50000000
0.71436250   0.02051967   0.50000000
0.28563750   0.97948033   0.50000000
```

IV. Mechanical properties

The mechanical features were investigated using the energy-strain method.[1,2] The strain energy per unit area can be expressed using the standard Voigt notation, as

$$U = \frac{1}{2}\, C_{11}\, \tau_x^2 + \frac{1}{2}\, C_{22}\, \tau_y^2 + \frac{1}{2}\, C_{12}\, \tau_x \tau_y + 2\, C_{66} \tau_{xy}^2,$$

where $\tau_x$ and $\tau_y$ represents the strain along x- and y-direction, and $\tau_{xy}$ are the shear strain. $C_{11}, C_{22}, C_{12}$ and $C_{66}$ are the elastic modulus tensor components. From a series of calculations of the structure under different strain and fitting the energy curves, the elastic constants are determined as: $C_{11} = 323\ \mathrm{J/m^2}, C_{22} = 336\ \mathrm{J/m^2}, C_{12} = 72\ \mathrm{J/m^2}$, and $C_{66} = 125\ \mathrm{J/m^2}$. These constants satisfy $C_{11}\, C_{22} - C_{12}^2 > 0$ and $C_{66} > 0$, which are needed for a 2D material to be mechanically stable. The Poisson's ratios with x- and y-directions being the transverse directions are $v_{xy} = C_{12}/C_{22} = 0.22$ and $v_{yx} = C_{12}/C_{11} = 0.22$. Moreover, based on the obtained elastic tensors, we calculated the in-plane Young's modulus and Poisson's ratio along an arbitrary direction employing the formulae:[3]

$$E(\theta) = \frac{C_{11}\, C_{22} - C_{12}^2}{C_{11} sin^4\, \theta + C_{22} cos^4\, \theta + \left(\frac{C_{11}C_{22} - C_{12}^2}{C_{66}} - 2C_{12}\right) cos^2\, \theta\, sin^2\, \theta},$$

$$\vartheta(\theta) = -\frac{\left(C_{11} + C_{22} - \frac{C_{11}C_{22} - C_{12}^2}{C_{66}}\right) cos^2\, \theta\, sin^2\, \theta - C_{12}(cos^4\, \theta + sin^4\, \theta)}{C_{11}\, sin^4\, \theta + C_{22}\, cos^4\, \theta + \left(\frac{C_{11}C_{22} - C_{12}^2}{C_{66}} - 2C_{12}\right) cos^2\, \theta\, sin^2\, \theta},$$

in which $\theta$ is the angle of the arbitrary direction and x-direction. As shown in Fig. S3 (a) and (b), different from graphene, PAI-graphene shows an anisotropic mechanical property. The largest in-plane Young's moduli are along x- and y-directions, and the smallest in-plane Young's moduli are along $\theta = 45 \times\ n\ (n = 1, 2, 3, 4)$ directions. Compared with graphene and three other low-energy haeckelite structures (ψ-graphene, phagraphene, and SW-graphene), PAI-graphene have large and anisotropic Young's modulus up to 320 $\mathrm{J/m^2}$.

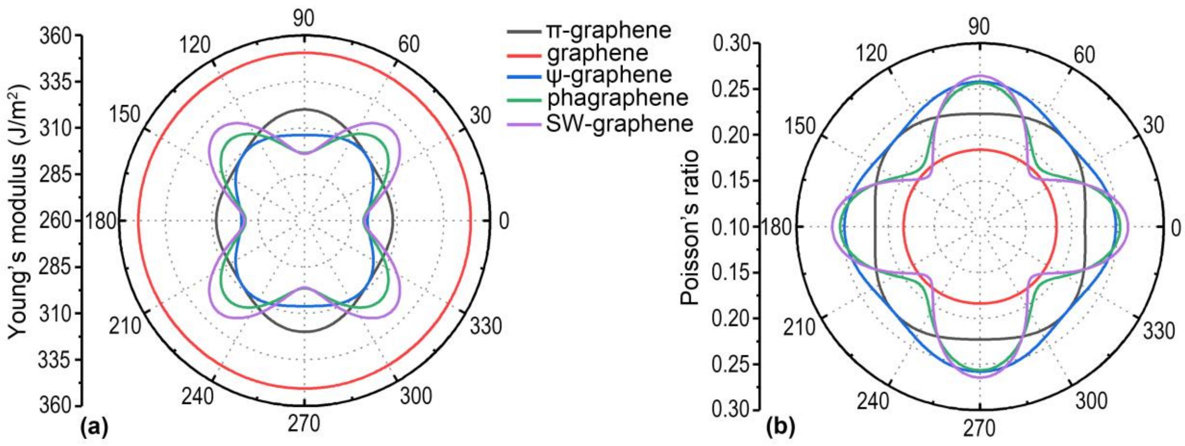


Figure S3 (a) and (b) is the comparison of the polar diagrams of Young's modulus and Poisson's ratio of PAI-graphene, graphene, ψ-graphene, phagraphene, and SW-graphene, respectively.

V. Electronic band structure and DOS by PBE calculation

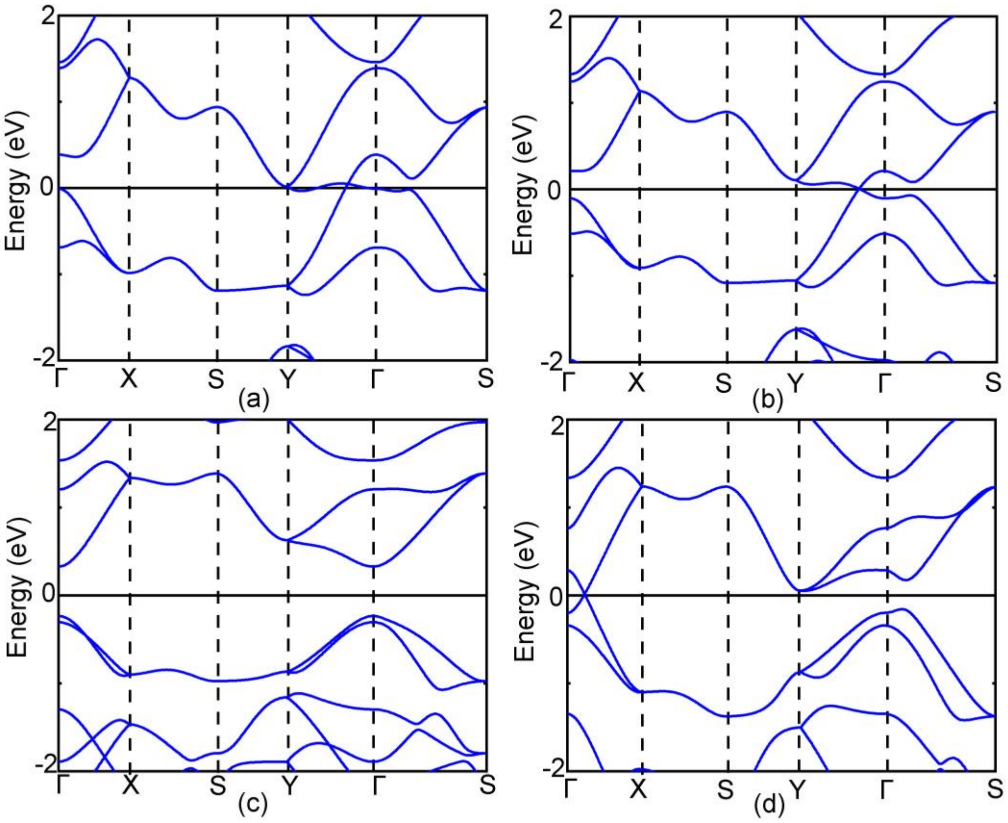


Figure S4 The electronic band structures of PAI-graphene (a) without and with strain of (b) $(\tau_x,\tau_y)$ = (5%,5%), (c) $(\tau_x,\tau_y)$ = (12%,15%), and (d) $(\tau_x,\tau_y)$ = (0%,10%), obtained by PBE.

VI. The character table of point group $D_{2h}$

| $D_{2h}$ | $E$ | $C_{2z}$ | $C_{2y}$ | $C_{2x}$ | $I$ | $\sigma_h$ | $m_y$ | $m_x$ |
|---|---|---|---|---|---|---|---|---|
| $\Gamma_1^+$ | 1 | 1 | 1 | 1 | 1 | 1 | 1 | 1 |
| $\Gamma_2^+$ | 1 | 1 | -1 | -1 | 1 | 1 | -1 | -1 |
| $\Gamma_3^+$ | 1 | -1 | -1 | 1 | 1 | -1 | -1 | 1 |
| $\Gamma_4^+$ | 1 | -1 | 1 | -1 | 1 | -1 | 1 | -1 |
| $\Gamma_1^-$ | 1 | 1 | 1 | 1 | -1 | -1 | -1 | -1 |
| $\Gamma_1^-$ | 1 | 1 | -1 | -1 | -1 | -1 | 1 | 1 |
| $\Gamma_1^-$ | 1 | -1 | -1 | 1 | -1 | 1 | 1 | -1 |
| $\Gamma_1^-$ | 1 | -1 | 1 | -1 | -1 | 1 | -1 | 1 |

Table S1. Character table of the point group $D_{2h}$.

VII. The phonon spectra of PAI-graphene under strain

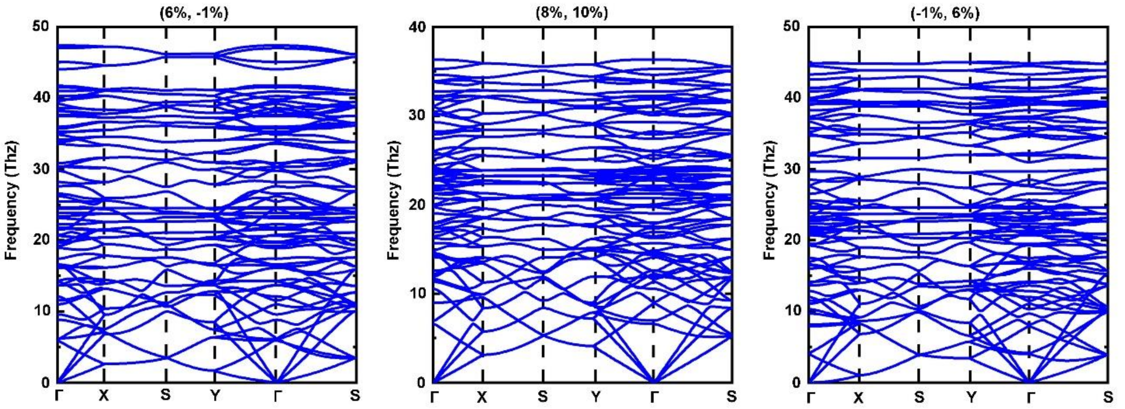


Figure S5 The phonon spectra of PAI-graphene with strain of $(\tau_x,\tau_y)$ = (6%, -1%), $(\tau_x,\tau_y)$ = (8%, 10%), and (d) $(\tau_x,\tau_y)$ = (-1%, 6%).

Reference


1. R. C. Andrew, R. E. Mapasha, A. M. Ukpong, and N. Chetty, Phys. Rev. B **85**, (2012) 125428. doi: 10.1103/PhysRevB.85.125428.
2. S. Zhang, J. Zhou, Q. Wang, X. Chen, Y. Kawazoe, and P. Jena Proc. Natl. Acad. Sci. U.S.A **112**, (2015) 2372. doi: 10.1073/pnas.1416591112.
3. E. Cadelano, P. L. Palla, L. Pier, S. Giordano, and L. Colombo, Phys. Rev. B **82**, (2010) 235414. doi: 10.1103/PhysRevB.82.235414.
